# Supplementary material for: CLASP: Constrained Latent Shape Projection for Refining Object Shape from Robot Contact
Source: arXiv:2110.08719 source file (2021-10-17)
Supplement: Supplementary file 1 [file ExtendedExperiments.tex]

% !TEX root = ../main.tex

\section{Further Experiment details}

\subsection{Generalizing of shape}

\begin{figure}[ht]
    \centering
    \includegraphics[width=0.99\textwidth]{images/training_similarity_recolored.png}
    \caption{Similarity to the Training shapes. Completions (Green) from a depth view (grey) are shown in both the top and bottom row. 
    In all cases the handle is occluded from the depth view.
    The top row additionally shows ground truth (transparent blue), while the bottom row additionally shows the training shape (orange) that is closest (chamfer distance) to the ground truth test shape. The completed handle is sometimes closer to the training shape (e.g. left-most), sometimes closer to the test shape (e.g. right-most) and sometimes different from both.
    }
    \label{fig:train_similarity}
\end{figure}
In addition to our main contribution, we ask if these shape completion networks are ``completing the shape" or ``looking up the closest object from the training set". 
To evaluate this we examine the quality of the completions of the test shape as compared to the \textit{training} shapes.
For each test shape from the Shapenet Mugs dataset we compute the closest (chamfer distance) training shape.
We then sample 10 completions from PSSNet using the 2.5D view of the test shape and compute chamfer distance to both the closest-training and test shapes. 
Over all 26640 samples, the average chamfer distance to the test and closest-train shapes are 2.4mm and 3.8mm respectively. 
We find that in 2599 (approx 10\%) of samples the completion is closer to the training shape.
Numerically this indicates PSSNet (and presumably other shape completion networks) are more than searching for the nearest shape.

Qualitatively we notice features, such as the mug handle, sometimes visually appear closer to the closest-training shape. 
We visualize selected instances in Figure \ref{fig:train_similarity}.
We note that visually these completions represent the diversity we desire, where the completion of an occluded handle can vary.

% \subsection{Additional Figures}
% \begin{figure}[h]
%     \centering
%     \includegraphics[width=0.99\textwidth]{images/ycb_completions.png}
%     \caption{Completions of YCB objects as viewed through a 6 pixel narrow slit with the nearest plausible shape shown for each network sample. The top row is a duplicate of \figref{fig:ycb_completions} for context, and the bottom row is a second example.}
%     \label{fig:ycb_completions_additional}
% \end{figure}

% \figref{fig:ycb_completions_additional} visualizes additional YCB completions to supplement \figref{fig:ycb_completions}

\subsection{Physical Robot Details} \label{sec:physical}
\begin{figure}
    \centering
    \includegraphics[width=0.99\linewidth]{images/robot_experiments_wide.png}
    % \caption{Robot grasping experiments for the mug (left) and Cheez-it box (right) with a sampled completion from $\ourmethod$.
    % The robot Kinect views the front while the above images were taken front back.}
    \caption{Robot scenarios for grasping Cheez-it box (top) and the mug (bottom).
    From left to right: The scene, the robot's view of the scene, 2 sampled completions using PSSNet, and a grasp attempt.}
    \label{fig:robot_appendix}
\end{figure}

We constructed two grasping scenarios on a physical robot, shown in \figref{fig:robot_appendix} and the accompanying video.
The points from a Kinect were filtered using an image segmenting network to construct known occupied and known free voxelgrids for the target object.
20 completions were sampled from which grasp poses were calculated, and then a grasp was attempted.
Our grasping strategies described below are simple but still serve to demonstrate the value of a diverse belief over shapes under ambiguity.

In the mug scenario, kinematics limits and clutter forced the robot to grasp the mug from the occluded handle on the far side from the robot.
For each completion a grasp was chosen with a handcoded orientation and grasp point as the furthest back possible grasp to avoid collision with other clutter.
The grasp attempted was the average of all valid grasp points with gripper width wide enough to capture all grasp points.
VAE-GAN sampled completions that did not have visible handles, resulting in most grasp poses in collision with other clutter.
Occasionally stray voxels appeared in VAE-GAN completions that generated valid grasp poses, but when attempted these grasps were not successful.
Using $\ourmethod$ sampled completions with handles generated valid grasps, which when executed resulted in successful grasps of the true mug.

In the Cheez-it scenario, clutter occluded all but a narrow slit from which only a small portion of the box was visible.
Potential grasps were sampled from both a top and side orientation with grasp point at the centroid of the completed object.
Completions from VAE-GAN were consistent, but the completed box was too shallow such that it appeared a top grasp would always be successful.
These attempted top grasps were unsuccessful because the gripper collided with the larger-than-expected box.
$\ourmethod$ again showed diversity with some completions thin and narrow and some as deep as the true box, so that it was unclear if a top grasp would be successful and thus the robot attempted and succeeded at side grasps.

% \todo{is this supposed to be plural? I though you only grabbed once.}.
% I grasped once for each trial
